# Supplementary material for: zkLogin: Privacy-Preserving Blockchain Authentication with Existing Credentials
Source: arXiv:2401.11735 source file (2024-09-27)
Supplement: Supplementary file 1 [file addr_derivation_extensions.tex]

\section{Other Address Derivation Options}
\label{sec:addr_derivation}

We describe certain trade-offs that need to be made depending on the type of identifier used.

\paragraph{Pairwise user identifiers} One solution is to simply derive a user's address from the pairwise ID. To be more precise, the address would be $H(\sub, \iss)$ where $\iss$ is the Provider's unique identifier.

But this means that the wallet is not interoperable (property 3b) as pairwise IDs are Relying-Party specific. 
For a similar reason, this solution also implies placing significant trust (property 4) in the Relying-Party.

An attractive alternative is to decide on a set of $n$ Relying Parties (or wallet) at account creation time such that the user can login from any of the $n$ wallets.
Then, the user's address is derived as $H((\sub_1, \aud_1), \ldots, (\sub_n, \aud_n), \iss )$.
In this way, we can mitigate the problems arising from the na\"ive solution to a large extent.

\paragraph{Public user identifiers} With public IDs, the interoperability challenges go away but a new set of issues arise, as we explain now. 
A starting solution could again be to derive a user's address from the public ID, e.g., $H(\sub, \iss)$. 

But this solution has some severe issues. 
First, we create a huge account security risk (property 4) because a single malicious Relying Party can, without the knowledge of a user, include an ephemeral key into the nonce and gain the ability to sign arbitrary transactions.
Second, this solution breaks unlinkability (property 5) because $\sub$ can be highly sensitive.\footnote{Even though most of the sensitive information in a JWT is not revealed, the link between the off-chain and on-chain identities is public.}

We resolve the first challenge by binding a user address to a set of wallets (like before).
The user decides on a set of $n$ Relying Parties and the user address is $H(\sub, (\aud_1, \aud_2, \ldots, \aud_n), \iss)$.

Coming to the second issue, namely unlinkability. First note that depending on what the public ID is and the user's preferences are, the privacy risk varies. For example, users might be willing to use their Twitch subject identifier (say) as opposed to their Google subject identifier (which is more audely used). 

We propose the following approach in case unlinkability is desired.
The idea is to use an additional \textit{linking secret}~$\pin$ to provide unlinkability. 
We derive a user's address as $\userAddress = H(\sub, (\aud_1, \aud_2, \ldots, \aud_n), \iss, \pin)$.
While this solution does involve an additional secret (violating the no-secrets property), we think it is acceptable because a well-designed UX can hide the existence of this secret from the user to the extent possible.
For example, we can rely on the relying party to store the linking secret so that the user does not need to enter it in their day-to-day interaction (the user only needs this secret in the corner cases, e.g., switching devices).

% \begin{table}[]
%     \centering
%     \begin{tabular}{c|c}
%          &  \\
%          & 
%     \end{tabular}
%     \caption{Caption}
%     \label{tab:approaches}
% \end{table}

\paragraph{Note} One could argue that as defined before, the property 4 (no additional trust) is weak because the OpenID Provider is still being trusted in all the solutions. 
One reason this can be important is if the Provider suddenly decides to disallow supporting blockchain wallets.
However, this can be easily overcome by deriving the address alternatively as follows, e.g., $H((\sub_1, \aud_1, \iss_1), \ldots, (\sub_n, \aud_n, \iss_n) )$, such that the user is able to access their account as long as one of the $n$ providers are live.
